# Supplementary material for: How Well Do Self-Supervised Methods Perform in Cross-Domain Few-Shot Learning?
Source: arXiv:2202.09014 source file (2025-01-25)
Supplement: Supplementary file 1 [file appendix.tex]

\begin{table}[h]
\centering
\begin{tabular}{lccccc}
\hline
\hline
{} & {LR} & {CC} & {SVM} & {NN} & {Proto}\\
\hline
{ChestX} & 3.35 & 8.35 & 7.61 & 7.60 & 8.15 \\
{ISIC} & 2.13 & 7.71 & 6.63 & 6.37 & 6.87 \\
{EuroSAT} & 2.09 & 6.31 & 5.12 & 4.99 & 6.18 \\
{CropDisease} & 1.78 & 6.21 & 6.10 & 6.95 & 8.03 \\
\hline
{average} & 2.34 & 7.14 & 6.36 & 6.48 & 7.31 \\
\hline
\end{tabular}
\caption{The average speed (number of iteration per second it/s) of each classifier during testing from all methods listed in Table\ref{tab:tabname4}. Four target datasets are used to get the final average speed.}
\label{tab:tabname5}
\end{table}
